# Supplementary material for: Cascaded Video Generation for Videos In-the-Wild
Source: arXiv:2206.00735 source file (2022-06-01)
Supplement: Supplementary file 1 [file appendix.tex]

\clearpage
\appendix

\subsection{Additional Implementation Details}
We use the Adam optimizer~\cite{kingma2014adam} with learning rate $\lambda_G = 1e10^{-4}$ and $\lambda_D = 5e10^{-4}$ for the generator and the discriminator, respectively. The discriminator is updated twice for each generator update.

We use orthogonal initialization for all the weights in our model and use spectral normalization both in the generator and the discriminator.
We only use the first singular value to normalize the weights.
We do not use weight moving averages nor orthogonal penalties. 

Conditional batch normalization layers use the input noise as the condition, concatenated with the  class label when applicable.
Features are normalized with a per-frame mean and standard deviation.

To unroll a generator beyond its training temporal horizon, we apply it convolutionally over longer input sequences.
We perform 200 ``dummy'' forward passes to recompute the per-timestep batch normalization statistics at test time.

All convolutions in our models use 3x3 or 3x3x3 filters with padding=1 and stride=1, for 2D or 3D convolutions respectively.
All models were implemented in PyTorch.

For the rest of the appendix, we use B to denote the batch size, T for the number of frames or timesteps, C for the number of channels, H for the height of the frame and W is the width of the frame.

\subsection{Model Architecture - First level architecture}

\paragraph{Generator}
The generator is composed by a stack of units where each unit is comprised of a ConvGRU layer and two 2D-ResNet upsampling blocks. 
We follow the nomenclature of~\cite{brock2018large, clark2019efficient} and describe our network using a base number of channels $ch$ and the channel multipliers associated with each unit. 
Our first level generator is formed by 4 units with channel multipliers $[8, 8, 4, 2]$. 
The base number of channel is $128$.

The first input of this network is of size BxTx(8x$ch$)x4x4.
This input is obtained by first embedding the class label onto a 128 dimensional space, then concatenating the embedding to a 128 dimensional noise vector. 
This concatenation is mapped to a Bx(8x$ch$)x4x4 tensor with a linear layer and a reshape, and then the final tensor is obtained by replicating the output of the linear layer T times.

The ConvGRU layer~\cite{ballas2015delving} follows the ConvGRU implementation of ~\cite{clark2019efficient} and uses a ReLU non-linearity to compute the ConvGRU update.

The 2D ResNet blocks are of the norm-act-conv-norm-act-conv style.
We use conditional batch normalization layers, ReLU activations and standard 2D convolutions.
Before the first convolution operation and after the first normalization and activation, there is an optional upsampling operation when increasing the resolution of the tensor.
We use standard nearest neighbor upsampling. 
Except for the last unit, all units perform this upsampling operation.
The conditional batch normalization layers receive the embedded class label (if applicable) and the input noise as a condition and map it to the corresponding gain and bias term of the normalization layer using a learned linear transformation.
The 2D ResNet blocks process all frames independently by reshaping their input to be (B*T)xCxHxW.

The output of the last stack goes through a final norm-relu-conv-tanh block that maps the output tensor to RGB space with values in the [-1, 1] range.

\paragraph{Discriminator}
There are two discriminators, a 2D spatial discriminator and a 3D temporal discriminator.
The 2D discriminator is composed of 2D ResNet blocks.
Each ResNet block is formed by a sequence of relu-conv-relu-conv layers.
There are no normalization layers in the discriminator.
After the last conv in each block there is an optional downsampling operation, which is implemented with average pooling layers.
The 2D discriminator receives as input 8 randomly sampled frames from real or generated samples.

The 3D discriminator is equal to the 2D discriminator except that its first two layers are 3D ResNet blocks, implemented by replacing 2D convolutions with regular 3D convolutions.
The 3D discriminator receives as input a spatially downsampled (by a factor of two) real or generated sample.
The 2D blocks process different timesteps independently.

We concatenate the output of both discriminators and use a geometric hinge loss.
The loss is averaged over samples and outputs.

We use $128$ as base number of channel for both discriminators, with the following channel multipliers for each ResNet block: $[16, 16, 8, 4, 2]$

\subsection{Model Architecture - Upsampling levels architecture}

The upsampling levels follow the same architecture as the first level but with the following modifications.

\paragraph{Generator}
The generator units replace the ConvGRU layers with a Separable 3D convolution. 
We first convolve over the temporal dimension with a 1D temporal kernel of size 3 and then convolve over the spatial dimension with 2D 3x3 kernel. 
We empirically compare generators with ConvGRU and separable convolutions in section~\ref{app:comparison}, showing that the 3D convolution performs as well as the ConvGRU but it can be run in parallel.

We add residual connections at the end of each 3D and 2D ResNet block to an appropriately resized version of $\mathbf{x}^{l-1}$.
We use nearest neighbor spatial downsampling for this operation, and we use nearest neighbor temporal interpolation to increase the number of frames of $\mathbf{x}^{l-1}$. We then map the residual to the appropriate number of channels using a linear $1$x$1$ convolution.
We do not add $\mathbf{x}^{l-1}$ residual connections to feature maps with spatial resolutions (HxW) greater than the resolution of $\mathbf{x}^{l-1}$.

\paragraph{Discriminator}
We reuse the same 2D and 3D discriminators as for the first stage.
Additionally, we add a matching discriminator that discriminates $(\mathbf{x}^{l}, \mathbf{x}^{l-1})$ pairs.
The matching discriminator utilizes the same architecture as the 3D discriminator.
It receives as input a concatenation of $\mathbf{x}^{l-1}$ and a downsampled version of $\mathbf{x}^{l}$ to match the resolution of $\mathbf{x}^{l-1}$.
We concatenate the outputs of all three networks and use a geometric hinge loss, as done for the first level discriminator.
The overall loss is averaged over samples and output locations.

For 128x128 generations on Kinetics, the generator uses $128$ as base number of filters with the following channel multipliers $[8, 8, 4, 2, 1]$. All discriminators have $96$ base channels and the following channel multipliers $[1, 2, 4, 8, 16, 16]$.
All our Kinetics models at 128x128 are two-level models.
We train models to upsample inputs of sizes 3/32x32 or 6/32x32 to 6/128x128 or 12/128x128, respectively.
Since we train our first level for 24/32x32 outputs, our two-level models can generate 48/128x128 outputs when unrolled.

For 128x128 generations on BDD100K, the generator uses $96$ as the base number of channels with channel multipliers $[8, 8, 4, 2, 1]$. 
All discriminators have $96$ base channels and channel multipliers $[1, 2, 4, 8, 16, 16]$.
Our BDD100K 128x128 models upsample 6/64x64 inputs to 12/128x128, and can generate outputs of up to 24/128x128. 

For 256x256 generations on BDD100K, the generator uses $96$ as the base number of channels with channel multipliers $[8, 4, 4, 4, 2, 1]$. 
All discriminators have $96$ base channels and channel multipliers $[1, 2, 4, 8, 8, 16, 16]$.
Our 256x256 model upsamples 6/128x128 inputs to 12/256x256, and can generate outputs of up to 48/256x256.

\subsection{Comparison of Recurrent Layers}
\label{app:comparison}

\begin{figure}
\begin{subfigure}{0.45\textwidth}
    \centering
    \includegraphics[width=\textwidth]{figures/normalized_fvd.png}
\end{subfigure}
\hfill
\begin{subfigure}{0.45\textwidth}
    \centering
    \includegraphics[width=\textwidth]{figures/normalized_is.png}
\end{subfigure}
\caption{\textbf{Comparison of recurrent layers} We compare two variants of the same generator, one with a single ConvGRU layer per generator block and one with a separable 3D convolution per generator block. 
On the left we show the evolution of the FVD score during training, and on the right we show the Inception Score.
Both scores are normalized to the [0, 1] range where 1 is the highest score obtained by these models and 0 the lowest.
Both models have similar behaviour and computational costs, but the 3D convolution processes inputs in parallel.}
\label{fig:appendix_conv3d}
\end{figure}

In this section we justify the change of the ConvGRU for Separable 3D convolutions in upsampling levels.
In Figure~\ref{fig:appendix_conv3d} we compare the evolution of two metrics (IS and FVD) during training for two variants of the same two-stage model, one using ConvGRUs and one using separable 3D convolutions.
Both models show similar behavior during training and achieve similar final metrics.
However, ConvGRUs perform sequential operations over time whereas 3D convolutions can be parallelized.

\clearpage
\subsection{Power Spectrum Density}

\begin{figure}[!b]
    \centering
    \includegraphics[trim={10 10 10 10}, clip, width=0.95\linewidth]{figures/psd_v2.png}
    \caption{\textbf{Power Spectrum Density (PSD) plots for different time steps} We show a comparison of the PSD between the original data and our generations at different steps in the predictions. We observe that our generations have a similar PSD to that of the original data, even at the end of the generation, indicating that the generations do not blur over time significantly.}
    \label{fig:psd}
\end{figure}

Some video generation models produce blurry results over time. 
As an additional evaluation, we generate Power Spectrum Density (PSD) plots to assess whether our generations become blurrier over time, following~\cite{ayzel2020rainnet}.

We conduct this experiment on Kinetics for videos of 48 frames at 128x128 resolution.
We use our model with the first level trained on 24/32x32 sequences and the second level trained to generate 12/128x128 video snippets from 6/32x32 windows, and unrolled after training to produce 48/128x128 videos.
We took 1800 random videos from the ground truth data (GT) and 1800 generations from our model.
We compute the PSD at frames 1, 10, 24, and 48 of each video.
For each set of 600 videos, we compute the average PSD across videos, on a per frame basis.
Finally, we use the three sets of 600 videos to compute the standard deviation and mean for the average PSD of the original data and our generations.
Figure~\ref{fig:psd} shows the plots for different frame indices. 
Our generations have a very similar PSD to that of GT in all video frames.
This indicates that our generations, while they might not be accurate, have very similar frequency statistics as the ground-truth data.
We do not observe any significant blurring over time, which is confirmed by the plots - they show that even for frame 48 high frequencies are very similar between the original data and our generations.

\subsection{Influence of Motion on the Results}

\begin{table}[ht]
    \centering
    \begin{tabular}{clccc}
    \toprule
    & & \multicolumn{2}{c}{48 frames} \\
    \cmidrule(lr){3-4} 
    & Class & IS ($\uparrow$) & FID  ($\downarrow$) & \# Videos \\
    \midrule
          \parbox[t]{2mm}{\multirow{5}{*}{\rotatebox[origin=c]{90}{\textbf{High Motion}}}} & Bungee Jumping & 11.66 & 82.21  & 799 \\
          & Capoeira       & 9.48  & 84.57  & 816 \\
          & Cheerleading   & 12.10 & 116.84 & 982 \\
          & Kitesurfing    & 11.36 & 108.81 & 648 \\
          & Skydiving      & 5.99  & 90.25  & 983 \\
    \midrule
          \parbox[t]{2mm}{\multirow{5}{*}{\rotatebox[origin=c]{90}{\textbf{Low Motion}}}} & Doing Nails  & 13.32 & 91.67  & 537 \\
          & Cooking Egg  & 7.60  & 111.63 & 441 \\
          & Crying       & 8.92  & 70.74  & 627 \\
          & Reading Book & 11.13 & 64.97  & 793 \\
          & Yawning      & 9.71. & 79.08  & 530 \\
    \bottomrule
    \end{tabular}
    \caption{\small \textbf{Per category scores for classes with different amounts of motion (Kinetics-600)} We report per-class IS and FID scores for 5 randomly selected categories with high motion and 5 categories with low motion. We observe that there is a high variability in FID scores, with some classes with low motion having high scores as well as some high motion classes. In IS scores there are few differences between the two groups, with the high motion group having a slightly higher mean score.}
    \label{tab:motion_metrics}
\end{table}

In this section we analyze whether our model has different performance for categories with different motion characteristics as an additional analysis. 

We conduct this experiment for \ourmodel trained on Kinetics-600 to generate 24/32x32 videos in the first level and then to upscale 6/32x326 videos to 12/128x128 videos for the second level. 
The second level is unrolled over the full first level generation to obtain 48/128x128 videos.

We randomly select five categories of videos with high motion content (bungee jumping, capoeira, cheerleading, kitesurfing and skydiving) and five categories with less dynamic videos (doing nails, cooking egg, crying, reading book and yawning).
We generate 1000 samples from \ourmodel for each category, and use all available samples in the dataset to compute IS and FID scores per category.

Table~\ref{tab:motion_metrics} shows the IS and FID scores of each class, while Figure~\ref{fig:samples_high_motion} and Figure~\ref{fig:samples_low_motion} show samples from high motion and low motion categories, respectively.
We do not observe a trend that indicates that \ourmodel produces worse generations for high motion classes. 
Some low motion categories have high FID scores similar to the highest scores for the high motion categories, while on average the IS scores for the high motion categories are slightly better.
We do not notice a qualitative difference.
Instead, we believe there might be other factors - amount of structure present in a scene for example -  that have greater impact on the output quality.

\begin{figure*}
    \centering
    \includegraphics[width=1.0\textwidth]{figures/high_motion.pdf}
    \caption{\textbf{Samples from Kinetics-600 classes with high motion content}}
    \label{fig:samples_high_motion}
\end{figure*}

\begin{figure*}
    \centering
    \includegraphics[width=1.0\textwidth]{figures/low_motion.pdf}
    \caption{\textbf{Samples from Kinetics-600 classes with low motion content}}
    \label{fig:samples_low_motion}
\end{figure*}

\clearpage
\subsection{Cascaded Training Objective}
In this section we describe our training objective more formally.
For a \ourmodel model with $L$ levels, our goal is to model the joint probability distribution $p_{d}(\mathbf{x}^1, ..., \mathbf{x}^L) = p_{g}(\mathbf{x}^1, ..., \mathbf{x}^L) = p_{g_L}(\mathbf{x}^L | \mathbf{x}^{L-1}) .. p_{g_1}(x^1)$, where each $p_{g_l}$ is defined by a level $l$ in our model.

\paragraph{Training Level 1} We consider the distribution $p_{g_1}$ and solve a min-max game with the following value function:
\begin{eqnarray*}
& V_1(G_1, D_1) = \\
& \mathbb{E}_{\mathbf{x}^1\sim p_{d}} [\log (D_1(\mathbf{x}^1))] + \mathbb{E}_{\mathbf{z}_1 \sim p_{z_1}} [\log (1-D_1(G_1(\mathbf{z}_1)))],
\end{eqnarray*} where $G_1$ and $D_1$ are the generator/discriminator associated with the first stage and $p_{z_1}$ is a noise distribution.

This is the standard GAN objective. As shown in~\cite{goodfellow2014generative}, the min-max game $\min_{G_1} \max_{D_1} V_1(G_1, D_1)$ has a global minimum when $p_{g_1}(\mathbf{x}^1) = p_{d}(\mathbf{x}^1)$.

\paragraph{Training upsampling levels} 
For each upscaling level $l > 1$ we formulate a min-max game with the following value function:
{\small
\begin{eqnarray*}
& V_l(G_l, D_l) = \\
&  \mathbb{E}_{\mathbf{x}^{l-1}, ..., \mathbf{x}^{1}\sim p_{d}} \mathbb{E}_{\mathbf{x}^l\sim p_{d}( .| \mathbf{x}^{l-1}, ..., \mathbf{x}^{1})} [\log(D_l(\mathbf{x}^{l}, \mathbf{x}^{l-1}))] + \nonumber \\ & \mathbb{E}_{\mathbf{\hat{x}}^{l-1}\sim p_{g_{l-1}}} \mathbb{E}_{\mathbf{z}_l\sim p_{z_l}} [\log(1-D_l(G_l(\mathbf{z}_l, \mathbf{\hat{x}}^{l-1}),  \mathbf{\hat{x}}^{l-1}))],
\end{eqnarray*}} where $G_l$, $D_l$ are the generator and discriminator of the current level and $p_{g_{l-1}}$ is the generative distribution of the level $l-1$.

The min-max game $\min_{G_l} \max_{D_l} V_l(G_l, D_l)$ has a global minimum when the two joint distributions are equal, $p_{d}(\mathbf{x}, ..., \mathbf{x}^l) = p_{g_l}(\mathbf{x}^l | \mathbf{x}^{l-1}) .. p_{g_1}(\mathbf{x}^1)$~\cite{dumoulin2016adversarially, donahue2016adversarial}. 
It follows that $p_{d}(\mathbf{x}^l | \mathbf{x}^{l-1}) = p_{g_l}(\mathbf{x}^l | \mathbf{x}^{l-1})$ when $p_{g_{l-1}}(\mathbf{x}^{l-1} | \mathbf{x}^{l-2}) .. p_{g_1}(\mathbf{x}^1) = p_{d}(\mathbf{x}^{l-1}, ..., \mathbf{x}^1)$.
Level $l$ only learns the parameters associated with the distribution $p_{g_l}$, as all $p_{g_i}, 1 \leq i \leq l-1 $ levels are trained previously and their training objectives admit a global minimum when they match the data distribution. 
However, even if the distribution $p_{g_{l-1}}$ does not match exactly the marginal data distribution, our model still aims at learning a distribution $p_{g_l}$ such that $p_{g_l}(\mathbf{x}^l | \mathbf{x}^{l-1}).. p_{g_1}(\mathbf{x}^1)$ approximates the joint data distribution.

\subsection{DVD-GAN unrolling}

\begin{figure*}[t]
    \centering
    \includegraphics[trim={0 80 0 0},clip,width=\textwidth]{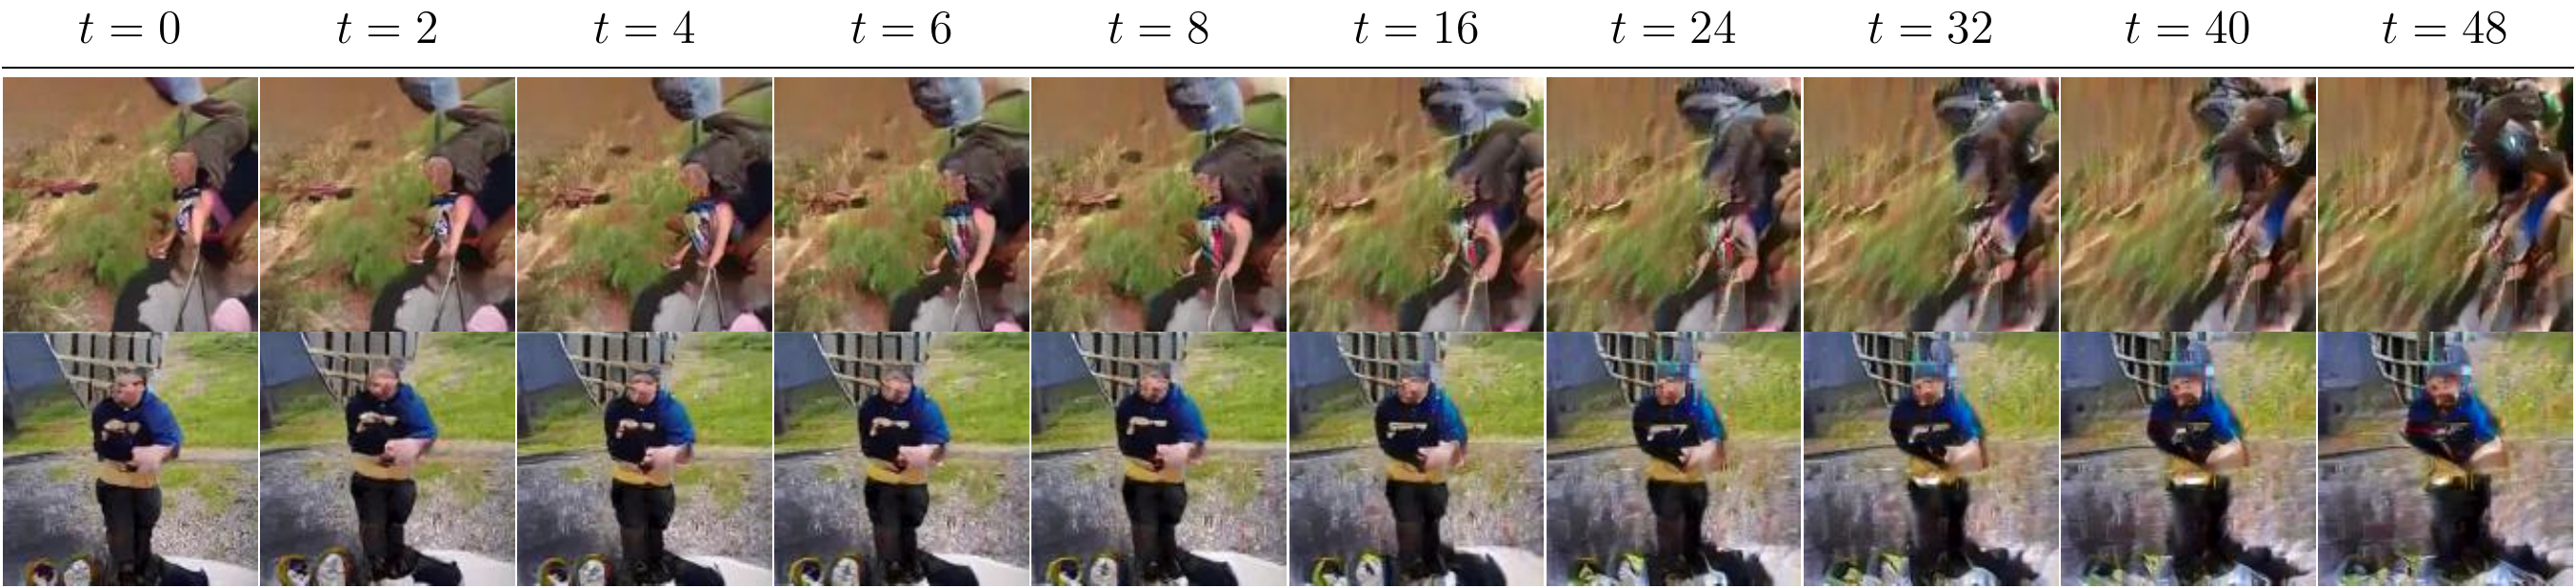}
    \caption{\small \textbf{DVD-GAN fails to generate samples beyond its training horizon}
    These samples were obtained by changing the spatial dimensions of the latent in a 6/128x128 \dvdgan model to produce 48/128x128 videos. The samples quickly degrade after the first few frames and become motionless.}
    \label{fig:dvdgan_unroll}
\end{figure*}

One of the main characteristics of \ourmodel is the ability to change the training and inference setup for upscaling levels.
Since \dvdgan is mostly a convolutional model, we investigate whether it can generate videos of longer duration than those it is trained on.
The number of frames in that model is controlled by the RNN that receives as input the latent variable sample and outputs as many tensors as frames to be generated.
We adjust the number of steps for this RNN and recompute batch normalization statistics to account for the extended amount of frames.
A prototypical example from an extended \dvdgan model generation can be found in Figure~\ref{fig:dvdgan_unroll}.
We observe that for this model videos are coherent up until the training length, but then they visibly degrade and quickly become motionless, producing implausible generations.

\subsection{Time Complexity}

\begin{table}[t]
\setlength{\tabcolsep}{2pt}
\centering
\small
    \begin{tabular}{lccc}
    \toprule
    & Iteration time & Total time \\
    \midrule
    \ourmodel Level 1  & 3.45s     & 4 days \\
    \ourmodel Level 2  & 3.20s     & 3.7 days \\
    DVD-GAN      & 11.90s    & 13.8 days \\
    \bottomrule
    \end{tabular}
    \caption{\small \textbf{Training time comparison}}
    \label{tab:time_complexity}
 \end{table}
 
In Table~\ref{tab:time_complexity} we compare a two-level \ourmodel and a \dvdgan model with similar capacity trained on 48/128x128 Kinetics-600 videos with a batch size of 512 and 64 GPUs. 
In addition to the memory savings, the total training time of \ourmodel (7.7 days) is significantly shorter.
Our approach uses smaller networks at each level and produces smaller outputs.  
Therefore, each level can have a reduced training iteration time. 
Using an additional third level to generate larger outputs increases the CVG training time. 
However, we cannot train the equivalent DVD-GAN baseline for the three-level model due to memory constraints, as it does not fit in GPU memory even with a batch size of 1 example.

\subsection{BDD100K metrics}

\begin{table*}[!h]
    \centering
    \begin{tabular}{cccccc}
    \toprule
    & & \multicolumn{2}{c}{Evaluated on 12 frames} & \multicolumn{2}{c}{Evaluated on 48 frames} \\
    \cmidrule(lr){3-4} \cmidrule(lr){5-6} 
    Model & Trained on & FID ($\downarrow$) & FVD ($\downarrow$)  & FID ($\downarrow$) & FVD ($\downarrow$) \\
    \midrule
    3-Level \ourmodel & 12/256x256 & 3.66 & 541.37 & 21.38 & 391.69 \\ 
    \bottomrule
    \end{tabular}
    \caption{\small \textbf{BDD100K 256x256 Metrics} We report the FID and FVD scores for our three-level \ourmodel trained on BDD100K. The model is trained to generate 12/256x256 videos and at inference it produces 48/256x256 videos.}
    \label{tab:bdd_256_metrics}
\end{table*}

We report the metrics for our three-level BDD100K model for help future comparison to \ourmodel in Table~\ref{tab:bdd_256_metrics}.

\paragraph{Qualitative comparison with \dvdgan}
As a point of comparison we provide samples from the official \dvdgan 48/128x128 trained on Kinetics-600 and released by the authors.
Samples can be download at this URL:  \url{https://drive.google.com/file/d/1P8SsWEGP6tEGPPNPH-iVycOlN6vpIgE8/view?usp=sharing}. 
We observe that the samples from \dvdgan and our \ourmodel model are of similar quality.

\subsection{Additional Samples}
\begin{figure*}[th]
    \centering
    \includegraphics[trim={0 80 0 0}, clip,width=0.95\linewidth]{figures/samples_kinetics_appendix_1.pdf}
    \caption{\textbf{Additional samples for Kinetics 12/128x128} We show additional samples from our two-level Kinetics 12/128x128 model unrolled to generate 48/128x128 videos.}
    \label{fig:samples_kinetics_appendix}
\end{figure*}

\begin{figure*}[ht]
    \centering
    \includegraphics[width=\linewidth]{figures/samples_bdd_stage3_256_appendix.pdf}
    \caption{\textbf{Additional samples for BDD 48/256x256} We show additional samples from our three-level BDD 48/256x256 model.}
    \label{fig:samples_bdd_appendix}
\end{figure*}

\begin{figure*}[ht]
    \centering
    \includegraphics[trim={0 0 0 0}, clip, width=0.85\textwidth]{figures/figure_samples_ucf_appendix.pdf}
    \caption{\textbf{Samples from our model trained on UCF101} We show samples from our 16/128x128 model trained on UCF101.}
    \label{fig:ucf_appendix}
\end{figure*}

\clearpage
\subsection{Upsampling Visualizations}
\begin{figure*}[ht]
    \centering
    \includegraphics[trim={0 65 0 0}, clip, width=0.85\textwidth]{figures/samples_upsampling.pdf}
    \caption{\textbf{Pairs of samples from stage 1 and their corresponding stage 2 output} We show a few examples from our 12/128x128 two-level model trained on Kinetics-600 and unrolled to generate 48/128x128 videos. For each example, we show the first level low resolution generation and the corresponding level 2 upsampling. Level 2 outputs refine the details of the first level generations but retain the overall scene structure.}
    \label{fig:appendix_upsampling}
\end{figure*}

In this section we show some examples of level 1 generations on Kinetics-600 for a 24/32x32 model, as well as the corresponding 48/128x128 generations from level 2 trained to upscale 6/32x32 windows to 12/128x128 and unrolled over the whole first level generation.
Examples are shown in Figure~\ref{fig:appendix_upsampling}, in which, for each example, we show the level 1 generation on the top row and the corresponding level 2 generation in the lower row.
We observe that the second level adds details and refines the low resolution generation beyond simple upsampling, but at the same time keeps the overall structure of the low resolution generation and is properly grounded.
